# Supplementary material for: A Generalized Read-Shockley Model and Large Scale Simulations for the Energy and Structure of Graphene Grain Boundaries
Source: arXiv:1611.06592 source file (2016-11-20)
Supplement: Supplementary file 1 [file SupplementaryInformation.pdf]

# Supporting Information for "A Generalized Read-Shockley Model And Large Scale Simulations For Graphene Grain Boundary Energy And Structure"

Ashivni Shekhawat[1,2,3], Colin Ophus[4], and Robert O. Ritchie[1,2]

[1]Department of Materials Science and Engineering, University of California Berkeley

[2]Materials Sciences Division, Lawrence Berkeley National Laboratory, Berkeley

[3]Miller Institute for Basic Research in Science, University of California Berkeley

[4]National Center for Electron Microscopy, Molecular Foundry, Lawrence Berkeley National Laboratory, Berkeley

## S1 Grain Boundary Burger's Vector

Consider the general grain boundary (GB) shown in Figure 1a of the main text. Let the operations $\mathbf{S}$, $\mathbf{S}'$ map the grains $\mathcal{G}$, $\mathcal{G}'$ onto some reference crystal. Let $\mathbf{v}_{\text{int}}$ be an unit interfacial vector along the interface between these two grains. Then, $\mathbf{S}\mathbf{v}_{\text{int}}$, $\mathbf{S}'\mathbf{v}_{\text{int}}$ give the mapping of the unit interfacial vector $\mathbf{v}_{\text{int}}$ in the reference crystal. Thus, the Burger's vector, per-unit length along the interface is given by

$$\mathbf{n} = (\mathbf{S} - \mathbf{S}')\mathbf{v}_{\text{int}}. \tag{S1}$$

This is the famous Frank-Bilby equation. Since the reference crystal is invariant under the operation of any members of its symmetry point group, more generally we can write

$$\mathbf{n} = (\mathbf{P}\mathbf{S} - \mathbf{P}'\mathbf{S}')\mathbf{v}_{\text{int}}, \tag{S2}$$

where $\mathbf{P}$, $\mathbf{P}'$ are members of the symmetry group of the reference crystal. Since the reference configuration is arbitrary, for convenience we take it to coincide with the grain $\mathcal{G}$, thus $\mathbf{S} = \mathbf{I}$, where $\mathbf{I}$ is the identity operator. Taking a coordinate system with the unit vector $\mathbf{e}_1$ parallel to the lat-

tice vector $v_1$ (Figure 1a of main text), we get $\mathbf{v}_{\text{int}} = R_{-\pi/2+(\theta_{\text{M}}-\theta_{\text{L}})/2}\mathbf{e}_1$, $\mathbf{S}' = R_{-\pi/2-(\theta_{\text{M}}+\theta_{\text{L}})/2}$ where $R_\theta$ represents a positive rotation by angle $\theta$, and $\theta_{\text{M}}$, $\theta_{\text{L}}$ are the misorientation angle and the line angle, respectively, as discussed in the main text. Since graphene lattice has a six-fold symmetry axis, $\mathbf{P}$, $\mathbf{P}'$ are of the form $R_{N\pi/3}$, where $N$ is an integer. Substituting these in Equation S2 and simplifying, we get

$$\mathbf{n} = \begin{cases} 2\sin(\theta_{\text{M}}/2)\,(\cos(\theta_{\text{L}}/2)\mathbf{e}_1 - \sin(\theta_{\text{L}}/2)\mathbf{e}_2) & \text{for } 0 \leq \theta_{\text{M}} \leq 30^\circ \\ 2\sin(60^\circ - \theta_{\text{M}}/2)\,(\cos(\theta_{\text{L}}/2)\mathbf{e}_1 - \sin(\theta_{\text{L}}/2)\mathbf{e}_2) & \text{for } 0 \leq \theta_{\text{M}} \leq 60^\circ, \end{cases} \tag{S3}$$

where we choose $\mathbf{P}$, $\mathbf{P}'$ to minimize the norm of $\mathbf{n}$.

# S2 Minimization Problem

Equation 1 of the main text can be expanded into following two scalar equations (assuming $\theta_{\text{M}}^0 < 30^\circ$)

$$2\delta n_1 + \delta n_2 - \delta n_3 = \quad 2\delta\theta_{\text{M}}\cos(\theta_{\text{M}}^0/2)\cos(\theta_{\text{L}}^0/2) - 2\delta\theta_{\text{L}}\sin(\theta_{\text{M}}^0/2)\sin(\theta_{\text{L}}^0/2), \tag{S4}$$

$$\sqrt{3}\delta n_2 + \sqrt{3}\delta n_3 = -2\delta\theta_{\text{M}}\cos(\theta_{\text{M}}^0/2)\sin(\theta_{\text{L}}^0/2) - 2\delta\theta_{\text{L}}\sin(\theta_{\text{M}}^0/2)\cos(\theta_{\text{L}}^0/2). \tag{S5}$$

These can be rewritten as follows for convenience of notation

$$2\delta n_1 + \delta n_2 - \delta n_3 = d_1, \tag{S6}$$

$$\delta n_2 + \delta n_3 = d_2, \tag{S7}$$

where

$$d_1 = \quad 2\delta\theta_{\text{M}}\cos(\theta_{\text{M}}^0/2)\cos(\theta_{\text{L}}^0/2) - 2\delta\theta_{\text{L}}\sin(\theta_{\text{M}}^0/2)\sin(\theta_{\text{L}}^0/2), \tag{S8}$$

$$d_2 = -2\delta\theta_{\text{M}}\cos(\theta_{\text{M}}^0/2)\sin(\theta_{\text{L}}^0/2)/\sqrt{3} - 2\delta\theta_{\text{L}}\sin(\theta_{\text{M}}^0/2)\cos(\theta_{\text{L}}^0/2)/\sqrt{3}. \tag{S9}$$

We can eliminate $\delta n_2$, $\delta n_3$, to get

$$\delta n_2 = \frac{d_1 + d_2}{2} - \delta n_1, \quad \delta n_3 = \frac{d_2 - d_1}{2} + \delta n_1. \tag{S10}$$

Thus, the constrained minimization problem given by Equation 2 of the main text can be written as the following unconstrained problem

$$\text{Min.} \quad c_1|\delta n_1| + c_2\left|\frac{d_1+d_2}{2} - \delta n_1\right| + c_3\left|\frac{d_2-d_1}{2} + \delta n_1\right|. \tag{S11}$$

This is a linear minimization problem, and can be solved trivially. The minimum occurs at either $\delta n_1 = 0$ or $\delta n_1 = (d_1+d_2)/2$ or $\delta n_1 = (d_1-d_2)/2$, and the corresponding values of the minima are $c_2|(d_1+d_2)/2| + c_3|(d_1-d_2)/2|$ or $c_1|(d_1+d_2)/2| + c_3|d_2|$ or $c_1|(d_1-d_2)/2| + c_2|d_2|$. In all cases it can be seen that the solution to the minimization problem posed by Equation 2 of the main text is of the following form

$$\gamma(\theta_\mathrm{M}^0 + \delta\theta_\mathrm{M}, \theta_\mathrm{L}^0 + \delta\theta_\mathrm{L}) = \gamma(\theta_\mathrm{M}^0, \theta_\mathrm{L}^0) + \frac{Gb}{4\pi(1-\mu)}\left(A_1|\delta\theta_\mathrm{M} + A_2\delta\theta_\mathrm{L}| + A_3|\delta\theta_\mathrm{M} + A_4\delta\theta_\mathrm{L}|\right), \tag{S12}$$

where $A_i's$ are suitable constants. The above equation can be specialized for symmetric boundaries by setting $\theta_\mathrm{L} = \delta\theta_\mathrm{L} = 0$ to get

$$\gamma(\theta_\mathrm{M}^0 + \delta\theta_\mathrm{M}, 0) = \gamma(\theta_\mathrm{M}^0, 0) + \frac{Gb}{4\pi(1-\mu)}\left(A_1|\delta\theta_\mathrm{M}|\right), \tag{S13}$$

where $A_1$ is a new effective constant. This has the same asymptotic form near $\theta_\mathrm{M}^0$ as the parametrization presented by Equation 3 of the main text.

### S2.1 Symmetric Low Angle GBs

The solution becomes much simpler for low angle grain boundaries with $\theta_\mathrm{L}^0 = \theta_\mathrm{M}^0 = \delta\theta_\mathrm{L} = 0°$. For this case we get $d_1 = 2\delta\theta_\mathrm{M}$, $d_2 = 0$. The solution $\delta n_1 = 0$ corresponds to energy of $(c_2+c_3)|\delta\theta_\mathrm{M}|$, while the solutions with $\delta n_1 = (d_1 \pm d_2)/2$ correspond to energy of $c_1|\delta\theta_\mathrm{M}|$. It is reasonable to assume that $(c_2+c_3) > c_1$, since physically $c_1, c_2, c_3$ should be roughly equal. Thus the perturbation corresponding the minimum energy leads to the solution $\delta n_1 = (d_1 \pm d_2)/2$, $\delta n_2 = \delta n_3 = 0$, which means that the low angle GBs only contain dislocations with Burger's vectors aligned along the $\mathbf{e}_1$ direction (as described in the main text).

### S2.2 Symmetric High Angle GBs

A similar analysis, accounting for the form of the Burger's vector at high angles (Equation S3), shows that under similar assumptions, it is energetically favorable to align the dislocation cores

with two out of the three directions (as described in the main text).

### S2.3 General GBs

The general expansion of the energy of a GB vicinal to a high symmetry (low $\Sigma$ CSL) GB is given by Equation S12. However, the most general functional form that has the correct asymptotic expansion, as well as satisfies all the symmetry requirements will be extremely complicated. Thus, we use the observation from the numerically measured GB energy (and the theoretical arguments provided before) that the GB energy varies slowly in the $\theta_{\mathrm{L}}$ direction, and that there seem to be two kinds of ridges (as discussed in the main text) to reduce the number of free parameters at a general cusp from four to two, and propose the form given by Equation 4 of the main text.

## S3 Numerical Fits

Figure Figure S1 shows the effect of including higher harmonics in the fits to symmetric GB energy by increasing $n$ in Equation 3 of main text. It can be seen that adding further harmonics has only a marginal effect on the quality of the fits.

Figure Figure S2 shows the effect of attempting to fit the symmetric GB to a Fourier series that does not have the correct form of the cusp singularity, i.e.,

$$\gamma_{\mathrm{sym}}(\theta_{\mathrm{M}}) = \frac{Gb}{4\pi(1-\mu)}\left(\Sigma_{i=0}^{n} p_i \cos 3i\theta_{\mathrm{M}}\right). \tag{S14}$$

It can be seen that even a series with $n = 50$ terms is not able to capture the sharp cusp singularity properly.

Finally, the fitting parameters for the best fit shown in Figure 4 of the main text are as follows: $p_{02} = -3.89 \times 10^{-3}$, $p_{04} = -1.04 \times 10^{-3}$, $p_{13} = -1.37 \times 10^{-3}$, $p_{20} = -3.96 \times 10^{-2}$, $p_{22} = -3.07 \times 10^{-4}$, $p_{24} = -4.70 \times 10^{-4}$, $p_{31} = -2.08 \times 10^{-3}$, $p_{33} = 1.50 \times 10^{-4}$, $p_{40} = 2.93 \times 10^{-2}$, $p_{42} = -1.61 \times 10^{-3}$, $p_{44} = 1.64 \times 10^{-5}$, $a_1^t = 1.08 \times 10^{-1}$, $a_1^s = 2.17 \times 10^{-1}$, $a_2^t = -2.61 \times 10^{-1}$, $a_2^s = 1.11$.

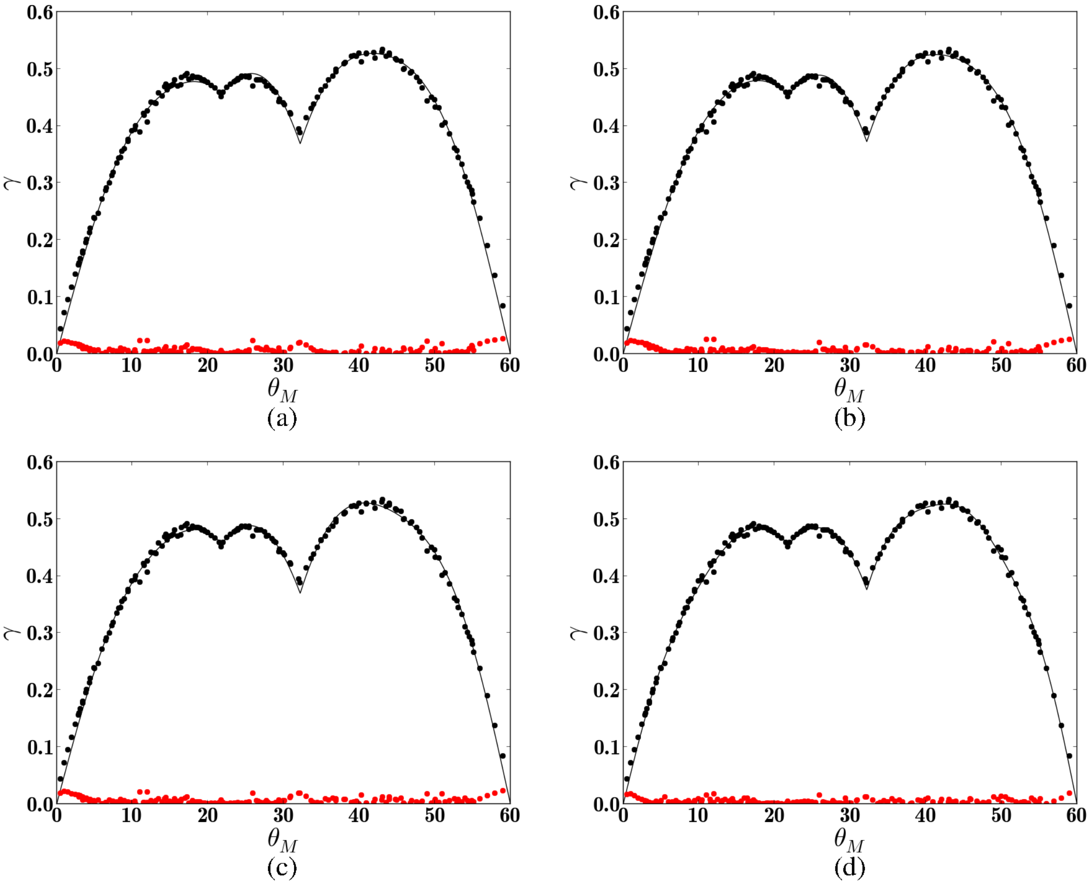


Figure S1: (Color Online) The fit of numerically measured GB energy for all symmetric GBs to Equation 3 of the main text with varying number of terms. (a), (b), (c), (d) correspond to $n = 4, 5, 6, 10$, respectively. It can be seen that the improvement on adding further harmonics is marginal. The filled black circles show the simulation data, while the solid line is a fit to Equation 3 of the main text. The filled red circles show the magnitude of the fitting error.

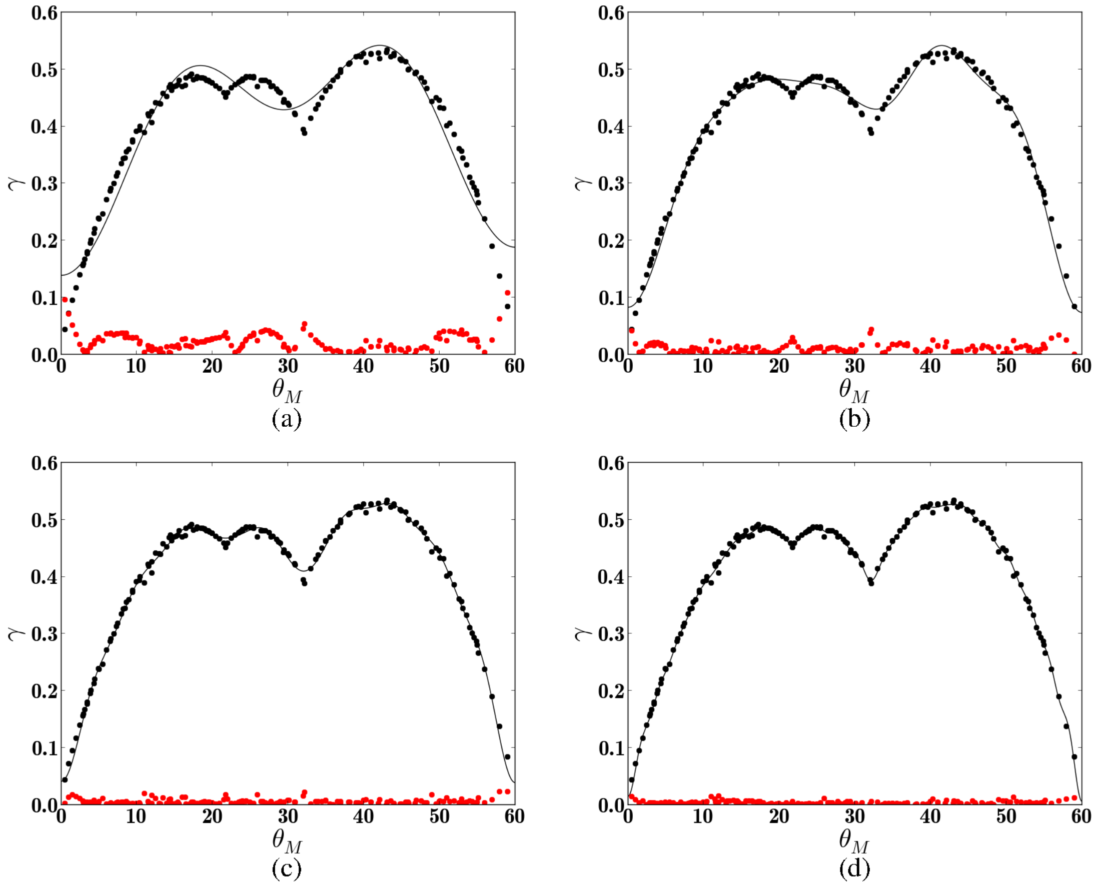


Figure S2: (Color Online) The fit of numerically measured GB energy for all symmetric GBs to Equation S14 with varying number of terms. (a), (b), (c), (d) correspond to $n = 4, 10, 20, 50$, respectively. It can be seen that a simple Fourier expansion without adding the correct asymptotic term for the cusps leads to very poor performance. Expansions with even 150 terms are not able to capture the singularity at the cusp effectively. The filled black circles show the simulation data, while the solid line is a fit to Equation S14. The filled red circles show the magnitude of the fitting error.

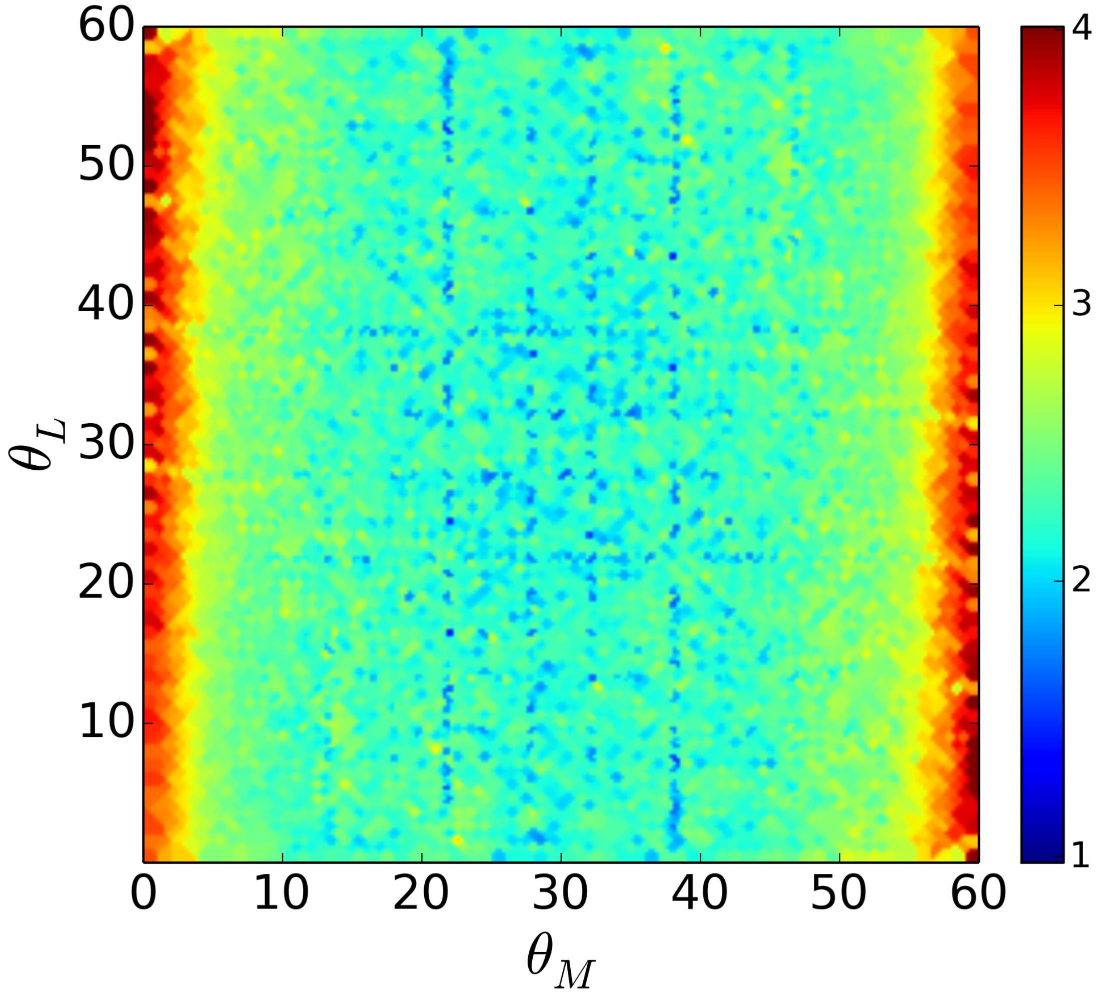


Figure S3: (Color Online) The maximum out of plane deformation in units of Å, as a function for the misorientation angle, $\theta_{\mathrm{M}}$, and the line angle $\theta_{\mathrm{L}}$.

## S4 Out Of Plane Deformation

Our simulations allow for unconstrained out of plane relaxation for the GB structures, since such relaxation is essential for lowering the energy of the structure. Figure Figure S3 the maximum out of plane displacement as a function of the misorientation angle and the line angle. It can be seen that the low angle grain boundaries have the largest out of plane displacement.
